# Supplementary material for: Balancing Label Imbalance in Federated Environments Using Only Mixup and Artificially-Labeled Noise
Source: arXiv:2409.13235 source file (2024-09-20)
Supplement: Supplementary file 1 [file supp_macros.tex]

\newcommand*{\mytensor}[1]{\bm{\mathcal{#1}}}
\newcommand*{\mymatrix}[1]{\bm{#1}}
\newcommand*{\myvector}[1]{\bm{#1}}
\newcommand*{\noise}[1]{\widehat{#1}}
\newcommand*{\mm}{\mymatrix}
\newcommand*{\mv}{\myvector}
\newcommand{\mt}{\mytensor}
\newcommand*{\mmCols}[2]{\mm{#1}_{[#2]}}

% names
\newcommand{\modname}{{TempLe}\xspace}
\newcommand{\modnamefull}{{Template Learning}\xspace}
\newcommand{\ourmod}{{O-TempLe}\xspace}
\newcommand{\ourmodfull}{{Online Template Learning}\xspace}
\newcommand{\ourmodtwo}{{FM-TempLe}\xspace}
\newcommand{\ourmodtwofull}{{Finite-Model Template Learning}\xspace}
\newcommand{\patnamefull}{{Transition Template}\xspace}
\newcommand{\patnamefulls}{{Transition Templates}\xspace}
\newcommand{\patnamelowercase}{{transition template}\xspace}
\newcommand{\patname}{\textsf{TT}\xspace}
\newcommand{\patnames}{\textsf{TT}s\xspace}
\newcommand{\patfunc}{{Templatize}\xspace}
\newcommand{\probgapname}{{ranking gap}\xspace}

% notations
\newcommand{\states}{\mathcal{S}}
\newcommand{\actions}{\mathcal{A}}
\newcommand{\pattern}{\mathbf{g}}
\newcommand{\patp}{\mathbf{g}^{(p)}}
\newcommand{\patr}{g^{(r)}}
\newcommand{\patsp}{g^{(p)}}
\newcommand{\pats}{g}
\newcommand{\patset}{\mathcal{G}}
\newcommand{\patvisset}{\mathcal{O}}
\newcommand{\patvis}{\mathbf{o}}
\newcommand{\patvisp}{\mathbf{o}^{(N)}}
\newcommand{\patvisr}{o^{(R)}}
\newcommand{\mdpset}{\mathcal{C}}
\newcommand{\permut}{\mathbf{\sigma}}
\newcommand{\dist}{\rho}
\newcommand{\thressm}{m_s}
\newcommand{\threslg}{m}
\newcommand{\mingap}{\omega}
\newcommand{\kset}{\mathcal{K}}

% algorithm2e
% \SetKwInput{Input}{Input}
% \SetKwInput{Output}{Output}
% \SetKwInput{Parameter}{Parameters}
% \SetKwFunction{Up}{Update}
% \SetKwFunction{Sin}{SingleRMax}
% \SetKwFunction{Pa}{Patternize}
% \SetKwProg{Fn}{Function}{:}{}

%algorithmic
\def\NoNumber#1{{\def\alglinenumber##1{}\State #1}\addtocounter{ALG@line}{-1}}
% \floatname{algorithm}{Algorithm}
% \renewcommand{\algorithmicrequire}{\textbf{Input:}}
% \renewcommand{\algorithmicensure}{\textbf{Output:}}
% previous
\newcommand{\dmname}{{dynamic matrix}\xspace}
\newcommand{\dmnames}{{dynamic matrices}\xspace}
\newcommand{\avgrew}{{AvgReward}\xspace}
\newcommand{\pavgrew}{{PostAvgReward}\xspace}
\newcommand{\numepi}{{TotalEps}\xspace}
\newcommand{\walkname}{{$\beta$-curious walking}\xspace}

%\newcommand{\noisebound}{\mathsf{gap}}
\newcommand{\coherence}{c_{\mathsf{max}}}
\newcommand{\gap}{\mathsf{gap}}
\newcommand{\op}{\mathsf{op}}
\newcommand{\diag}{\mathsf{Diag}}
\newcommand{\identity}{\mathbf{\mathds{1}}}
\newcommand{\identitymatrix}{\mm{I}}
\newcommand\R{\mathbb{R}}
\newcommand\BlkDiagFFT{\mathbf{\Theta}}
\newcommand\SuperLong{\mathsf{\sigma}}
\newcommand\defeq{\mathrel{\overset{\makebox[0pt]{\mbox{\normalfont\tiny\sffamily def}}}{=}}}
\newcommand\CirOneD{\mathsf{Cir_{1\!-\!d}}}
\newcommand\CirTwoD{\mathsf{Cir_{2\!-\!d}}}
\newcommand\DFTOneD{\mathsf{DFT_{1\!-\!d}}}
\newcommand\DFTTwoD{\mathsf{DFT_{2\!-\!d}}}
\newcommand\vectorize{\mathsf{flat}}
\newcommand{\Mod}[1]{\ (\text{mod}\ #1)}
\newcommand\CCir{\mathsf{Blk}\CirTwoD}

\def\viz{{viz.,\ \/}}
\newcommand{\suchthat}{\, \mid \,}
\def\Pbb{{\mathbb P}}
\def\Rbb{\mathbb{R}}
\def\Ebb{\mathbb{E}}
\def\tha{{\mbox{\tiny th}}}
\def\beq{\begin{equation}}
\def\bfI{{\mathbf I}}
\def\nn{\nonumber}
\def\eeq{\end{equation}\noindent}
\def\ci{\perp\!\!\!\perp} % from Wikipedia
\def\bfU{{\mathbf U}}
\newcommand{\redt}{\textcolor[rgb]{1,0,0}}
\newcommand{\bluet}{\textcolor[rgb]{0,0,1}}
\newcommand{\greent}{\textcolor[rgb]{0,1,0}}
\newcommand*{\conj}[1]{\overline{#1}}
\newcommand*{\hermconj}{^{\mathsf{H}}}


\newcommand{\bp}{\begin{psfrags}}
\newcommand{\ep}{\end{psfrags}}
\newcommand{\bc}{\begin{center}}
\newcommand{\ec}{\end{center}}

\newcommand{\llvert}{\left\vert\vphantom{\frac{1}{1}}\right.}
\newcommand{\xcmd}[2]{\left(#1\,\left\vert\vphantom{#1#2}\right. #2\right)}
\newcommand\independent{\protect\mathpalette{\protect\independenT}{\perp}}
\def\independenT#1#2{\mathrel{\rlap{$#1#2$}\mkern2mu{#1#2}}}

\newcommand*{\tcr}[1]{\textcolor{red}{#1}}
\newcommand*{\tcb}[1]{\textcolor{blue}{#1}}
\newcommand*{\textcal}[1]{%
  % family qzc: Font TeX Gyre Chorus (package tgchorus)
  % family pzc: Font Zapf Chancery (package chancery)
  \textit{\fontfamily{qzc}\selectfont#1}%
}
\newcommand{\shift}{\mathsf{Shift}}
\newcommand{\circshift}{\mathsf{Circshift}}
\newcommand{\ranktest}{\mathsf{RankTest}}
\newcommand{\sentence}{P}
\newcommand{\patch}{\mathcal{P}}

\newcommand{\Conv}{\mathop{\scalebox{1.5}{\raisebox{-0.2ex}{$\ast$}}}}%
\newcommand{\Toep}{\mathsf{Cir}}
\newcommand{\Cir}{\mathsf{Cir}}
\newcommand{\BCir}{\mathsf{BlkCir}}
\newcommand{\CToep}{{\mathcal{F}}}
%\newcommand{\CCir}{{\mathcal{F}}}
\newcommand{\Diag}{\mathsf{Diag}}
\newcommand{\Pair}{\mathsf{Pair}}
\newcommand{\Trip}{\mathsf{Trip}}
\newcommand{\Rank}{\mathsf{Rank}}
\newcommand{\DFT}{\mathsf{FFT}}

\newcommand*{\tran}{^{\mkern-1.5mu\mathsf{T}}}


\DeclarePairedDelimiter{\ceil}{\lceil}{\rceil}
\newcommand{\fro}{\mathsf{F}}
\DeclareMathOperator{\flatten}{unfold}
\DeclareMathOperator{\modeA}{\mathcal{F}}
\DeclareMathOperator{\modeB}{\mathcal{G}}
\DeclareMathOperator{\modeC}{\mathcal{H}}

\DeclareMathOperator{\basisV}{V_{basis}}

\DeclareMathOperator{\stationaryV}{v}
\DeclareMathOperator{\basis}{b}
\DeclareMathOperator{\coeff}{c}
\DeclareMathOperator{\errorTensor}{\mathcal{E}}
\DeclareMathOperator{\Cum}{C_3}
\DeclareMathOperator{\mat}{mat}
\DeclareMathOperator{\newCum}{M}
\DeclareMathOperator{\Fbb}{\mathbb{F}}
\DeclareMathOperator{\opt}{opt}
\DeclareMathOperator{\block}{blk}
\DeclareMathOperator{\blkdiag}{Blkdiag}
\DeclareMathOperator{\Tr}{\mathsf{trace}}
\DeclareMathOperator{\poly}{poly}
\def\calT{{\mathcal{ T}}}
%\newcommand{\fix}{\marginpar{FIX}}
%\newcommand{\new}{\marginpar{NEW}}
%%%%%%%%% new theoretical guaranteed symbols %%%%%%%%%%
\DeclareMathOperator{\onefilter}{f}
\DeclareMathOperator{\cirf}{\mathcal{F}}

\newtheorem{theorem}{Theorem}
\newtheorem{lemma}[theorem]{Lemma}
\newtheorem{definition}[theorem]{Definition}
\newtheorem{proposition}[theorem]{Proposition}
\newtheorem{corollary}[theorem]{Corollary}
\newtheorem{property}[theorem]{Property}
\newtheorem{condition}{Condition}
\newtheorem{fact}[theorem]{Fact}
\newtheorem{myfact}{Fact}
\newtheorem{assumption}{Assumption}
\floatname{algorithm}{Algorithm}
%\renewcommand{\algorithmicxrequire}{\textbf{Input:}}
%\renewcommand{\algorithmicxensure}{\textbf{Output:}}
% \makeatletter
% \def\thm@space@setup{%
%   \thm@preskip=0.3em
%   \thm@postskip=0.2em % or whatever, if you don't want them to be equal
% }
% \makeatother

\newcommand\FFTratio{\mathbf{\Gamma}}

\newcommand{\yc}{\textcolor[rgb]{0,0,1}{YC: }\textcolor[rgb]{0,0,1}}
\newcommand{\fh}[1]{\textcolor[rgb]{1,0,0}{[FH: #1]}} 
\newcommand{\tr}{\textcolor[rgb]{0,0,1}{TR: }\textcolor[rgb]{0,0,1}}
\newcommand{\br}[1]{\textcolor[rgb]{1,0,1}{[Brandon: #1]}} 

\colorlet{soulcyan}{cyan!30}
\DeclareRobustCommand{\hlcyan}[1]{{\sethlcolor{soulcyan}\hl{#1}}}
